# Supplementary material for: Breast Cancer Detection through Electrical Impedance Tomography and Optimal Control Theory: Theoretical and Computational Analysis
Source: arXiv:1809.05936 source file (2018-09-16)
Supplement: Supplementary file 1 [file Appendix1.tex]

\section{Optimal Regularity of Discretized Gradients via Preconditioning}
\label{sec:tuning_precond}

The discussed at length in \cite{Bukshtynov11} and \cite{Bukshtynov13} problem of improper suitability of $L_2$
gradients for the reconstruction of material properties may be in fact seen in the present problem due to lacking
necessary smoothness in gradients $\nabla_{\sigma} \mJ$ obtained by \eqref{eq:Frechet_Derivative}.
Figure~\ref{fig:grad_precond}(a) shows the spatial structure of gradient $\nabla_{\sigma} \mJ$ computed at
initialization of the optimization process, $N=0$, i.e.~for $\sigma^0 = \sigma_{ini}$ and $U^0 = U_{ini}$.
The problem of loosing regularity is clearly observed only at the parts of domain $Q$ close to its boundary $\partial Q$,
while in the interior region the shape of gradient $\nabla_{\sigma} \mJ$ does not show any signs of this problem.
The close view of this irregularity is presented in Figure~\ref{fig:grad_precond}(b) where the thin blue line depicts
the trace of the same gradient $\nabla_{\sigma} \mJ$ over boundary $\partial Q$ which contains multiple high
amplitude oscillations. The analysis of the shape of this trace and the location of these oscillations makes
a clear link to the structure of electrodes $E_l$. This also allows to make a conclusion that loosing regularity
of gradients $\nabla_{\sigma} \mJ$ is enforced by irregularity of solution $u(x; \sigma, U)$ as a result of
the imposed mixed-type boundary conditions \eqref{eq:forward_2}--\eqref{eq:forward_3}.
\begin{figure}[!htb]
  \begin{center}
    \mbox{
  \subfigure[]{\includegraphics[width=0.50\textwidth]{Figs/grad_full}}
  \subfigure[]{\includegraphics[width=0.50\textwidth]{Figs/grad_bound_precond}}}
  \caption{(a) Spatial structure of the gradient $\nabla^{L_2}_{\sigma} \mJ$ computed for $\sigma^0 = \sigma_{ini}$ and
    $U^0 = U_{ini}$.
    (b) Comparison of boundary traces of (blue thin line) the $L_2$ gradient $\nabla^{L_2}_{\sigma} \mJ$ and the Sobolev
    gradients $\nabla^{H^1}_{\sigma} \mJ$ defined by solving \eqref{eq:helm} for different values of preconditioning coefficient
    (thick blue line) $\ell = 10^{-5}$, (thick red line) $\ell = 10^{-4}$, and (thick pink line) $\ell = 10^{-3}$ computed
    for $\sigma^0 = \sigma_{ini}$ and $U^0 = U_{ini}$.}
  \label{fig:grad_precond}
  \end{center}
\end{figure}

One of the known approaches to eliminate negative impact of such irregularity, when a gradient method is implemented numerically,
is to derive an equivalent formula for the gradient with higher regularity. This idea is based on the Riesz representation theorem \red{[Berger, 1977]}, which expresses the isometrical isomorphism between a Hilbert space and its dual space if the underlying field
is the real numbers, see also \red{[Abdulla et al., 2018]} for details. Pursuing higher regularity, cost functional gradients
should be elements of $H^1(Q)$ space. Using isomorphism between the Sobolev space $H^1(Q)$ and $L_2(Q)$ space where our gradients
$\nabla^{L_2}_{\sigma} \mJ$ are initially obtained, one could project $\nabla^{L_2}_{\sigma} \mJ$ onto Sobolev space $H^1(Q)$
obtaining gradients $\nabla^{H^1}_{\sigma} \mJ$ with improved regularity. Following this idea, the Frechet differential could
be expressed in two different forms
\begin{equation}
  \begin{aligned}
    \delta \mJ(\sigma, U; \delta \sigma) &= \big< \nabla_{\sigma}^{L_2} \mJ, \, \delta \sigma \big>_{L_2(Q)}
    &&= \int_Q \nabla_{\sigma}^{L_2} \mJ \, \delta\sigma \, dx\\
    &= \big< \nabla_{\sigma}^{H^1} \mJ, \, \delta \sigma \big> _{H^1(Q)}
    &&= \int_Q \left[ \nabla_{\sigma}^{H^1} \mJ \, \delta\sigma +
    \ell \, \dfrac{d (\nabla_{\sigma}^{H^1}\mJ)}{dx} \dfrac{d (\delta \sigma)}{dx} \right] \, dx
    \end{aligned}
    \label{eq:dJ_L2_H1}
\end{equation}
in which $\ell \in \RR^+$ is a ``smoothing'' parameter; we note that the $L_2$ inner product is recovered by setting
$\ell = 0$ in \eqref{eq:dJ_L2_H1}. We perform integration by parts under assumption that Sobolev gradients
$\nabla_{\sigma}^{H^1} \mJ$ must satisfy homogeneous Neumann boundary conditions at $\partial Q$. Also by
noting that relation \eqref{eq:dJ_L2_H1} must be satisfied for any arbitrary $\delta \sigma$, we end up by determining
Sobolev gradients $\nabla_{\sigma}^{H^1} \mJ$ as a solution of the following inhomogeneous elliptic boundary--value problem
\begin{equation}
  \begin{aligned}
  \nabla_{\sigma}^{H^1} \mJ - \ell \, \frac{d^2}{dx^2} \nabla_{\sigma}^{H^1} \mJ & = \nabla_{\sigma}^{L_2} \mJ,
  \qquad && x \in Q \\
  \frac{\partial}{\partial n} \nabla_{\sigma}^{H^1} \mJ & = 0. && x \in \partial Q
  \end{aligned}
  \label{eq:helm}
\end{equation}
By changing the value of smoothing parameter $\ell$ we can control the smoothness of gradients $\nabla_{\sigma}^{H^1} \mJ$,
and therefore also the regularity of $\sigma(x)$. This technique in numerical optimization is also referred to as
{\it preconditioning}. More specifically, as was shown in \cite{gao2004improved}, extracting cost functional gradients
in the Sobolev spaces $H^p$, $p>0$, is equivalent to applying a low--pass filter to $L_2$ gradients with quantity $\ell$
representing the ``cut-off'' scale.
\begin{figure}[!htb]
  \begin{center}
  \mbox{
  \subfigure[]{\includegraphics[width=0.50\textwidth]{Figs/precond_obj}}
  \subfigure[]{\includegraphics[width=0.50\textwidth]{Figs/precond_sol_norm}}}
  \caption{(a) Cost functional $\mJ$ values and (b) solution norms
    $N_{\sigma} = \frac{\| \sigma - \sigma_{true}\|_{L_2}}{\| \sigma_{true}\|_{L_2}}$ and
    $N_U = \frac{\| U - U_{true}\|_{L_2}}{\| U_{true}\|_{L_2}}$ evaluated at termination (dots) for different
    values of preconditioning parameter $\ell$ and (dashed lines) without preconditioning ($\ell=0$).
    The best results obtained at $\ell^*_1 = 10^{-6}$ and $\ell^*_2 = 1.78 \cdot 10^{-8}$ are shown by hexagons.}
  \label{fig:precond_opt}
  \end{center}
\end{figure}

Similarly to PCA-based re-parameterization in Section~\ref{sec:tuning_pca}, performance of preconditioning is evaluated
first by examining cost functional $\mJ$ values while terminating computations for our benchmark ``voltage--to--current''
model described in Section~\ref{sec:tuning}. The outcomes with respect to different values of preconditioning parameter $\ell$
(blue dots) are shown in Figure~\ref{fig:precond_opt}(a). Dashed line represents the result of optimization without
preconditioning, i.e.~when $\ell=0$. First, we conclude that the effect of preconditioning is seen when $\ell < 10^{-4}$.
It is consistent with the results observed in Figure~\ref{fig:grad_precond}(b) that confirms that gradients preconditioned
with $\ell > 10^{-4}$ are loosing their informativeness. Second, we have to admit that when $\ell < 10^{-4}$ the effect of
preconditioning does not have any noticeable structure which may help to identify optimal value for $\ell$ parameter. We
pick two values (shown by hexagons) for the best results obtained at $\ell^*_1 = 10^{-6}$ and $\ell^*_2 = 1.78 \cdot 10^{-8}$.
Then we examine additionally $\sigma$ and $U$ solution norms
$N_{\sigma} = \frac{\| \sigma - \sigma_{true}\|_{L_2}}{\| \sigma_{true}\|_{L_2}}$ and
$N_U = \frac{\| U - U_{true}\|_{L_2}}{\| U_{true}\|_{L_2}}$ presented in Figure~\ref{fig:precond_opt}(b) with points for
results obtained at $\ell^*_1$ and $\ell^*_2$ also shown by hexagons. The maximum of the performance, seen at $\ell^*_1 = 10^{-6}$,
is evaluated as $1.65\%$ and $0.38\%$ in terms of improving solutions for $\sigma(x)$ and $U$ respectively.
