# Supplementary material for: Breast Cancer Detection through Electrical Impedance Tomography and Optimal Control Theory: Theoretical and Computational Analysis
Source: arXiv:1809.05936 source file (2018-09-16)
Supplement: Supplementary file 2 [file Appendix2.tex]

\section{Optimal Regularity of Discretized Gradients via Smoothed Boundary Conditions}
\label{sec:bc_smoothing}

As shown previously in Section~\ref{sec:kappa_test}, discretized gradients $\nabla_{\sigma} \mJ(\sigma,U)$ and
$\nabla_U \mJ(\sigma,U)$ are correct and consistent with their continuous representations given by \eqref{eq:Frechet_Derivative}.
We also noted that gradients $\nabla_U \mJ(\sigma,U)$ are obtained with much larger error in comparison to error
seen in $\nabla_{\sigma} \mJ(\sigma,U)$.
We explain this by the fact that computing gradients $\nabla_U \mJ(\sigma,U)$ relies mainly on the solution for
the potential $u(x)$ obtained on or very close to boundary $\partial Q$ where it looses its regularity due to
discontinuous boundary conditions \eqref{eq:forward_2}--\eqref{eq:forward_3}. One of the possible remedies to this
problem is to consider a new (combined) boundary condition in the following form
\begin{equation}
  \sigma(x) \Dpartial{u(x)}{n} = \chi_{\epsilon,l}(\theta) \dfrac{U_{l}-u(x)}{Z_l}, \quad l= \overline{1,m},
  \label{eq:new_BC}
\end{equation}
where $\chi_{\epsilon,l}(\theta)$ is a function used to ``smoothen'' boundary conditions \eqref{eq:forward_2}--\eqref{eq:forward_3}
with different degree of smoothness depending on value of parameter $\epsilon \geq 0$
\begin{equation}
  \chi_{\epsilon,l}(\theta) = \dfrac{1}{2} - \dfrac{1}{2} \tanh \dfrac{|\theta - \theta_{c,l}| - w}{\epsilon},
  \quad l= \overline{1,m}.
  \label{eq:chi}
\end{equation}
In the last formula $w$ is the half-width of electrode $E_l, \, l = 1, \ldots, m$, with its center positioned
at $\theta_{c,l}$, and $0^\circ \leq \theta < 360^\circ$ is an angular coordinate.
\begin{figure}[!htb]
  \begin{center}
  \mbox{
  \subfigure[]{\includegraphics[width=0.50\textwidth]{Figs/bc_smooth_approx}}
  \subfigure[]{\includegraphics[width=0.50\textwidth]{Figs/grad_bound_bc_smooth}}}
  \caption{(a) Function $\chi_{\epsilon,l}(\theta)$ given by \eqref{eq:chi} evaluated for
    (black line) $\epsilon = 0$, (blue line) $\epsilon = 10^{-2}$, (red line) $\epsilon = 5 \cdot 10^{-2}$,
    and (pink line) $\epsilon = 10^{-1}$. All cases are plotted using $l = 1, 2$, i.e.~for electrodes $E_1$ and $E_2$.
    (b) Comparison of boundary traces of gradient $\nabla_{\sigma} \mJ$ over boundary $\partial Q$ obtained
    for (thin blue line) $\epsilon = 0$, (think red line) $\epsilon = 5 \cdot 10^{-2}$, and (thick pink line)
    $\epsilon = 10^{-1}$.}
  \label{fig:bc_smooth}
  \end{center}
\end{figure}

Figure~\ref{fig:bc_smooth}(a) shows the shape of function $\chi_{\epsilon,l}(\theta)$ for different values of
$\epsilon = 0, 10^{-2}, 5 \cdot 10^{-2}, 10^{-1}$ evaluated for $l = 1, 2$, i.e.~for two first electrodes $E_1$ and $E_2$.
We note that setting $\epsilon = 0$ allows $\chi_{\epsilon,l} = 1$ for all $\theta$ corresponding to $E_l$ zones on boundary
$\partial Q$ and $\chi_{\epsilon,l} = 0$ for all $\theta$ corresponding to zones $\partial Q - \bigcup\limits_{l=1}^{m} E_l$,
which is shown by black line in Figure~\ref{fig:bc_smooth}(a). This, in fact, recovers original mixed boundary conditions \eqref{eq:forward_2}--\eqref{eq:forward_3}. Similar to Figure~\ref{fig:grad_precond}(b), Figure~\ref{fig:bc_smooth}(b) shows
the boundary traces of gradients $\nabla_{\sigma} \mJ$ over boundary $\partial Q$ obtained for different values of smoothing
parameter $\epsilon$ to confirm the effect of improving regularity for discretized gradients $\nabla_{\sigma} \mJ$.

Similarly to analysis performed in Sections~\ref{sec:tuning_pca}--\ref{sec:tuning_precond}, performance of smoothing mixed
boundary conditions discussed in this Section is evaluated by examining cost functional $\mJ$ values while terminating
computations for our benchmark ``voltage--to--current'' model described in Section~\ref{sec:tuning}. The outcomes with respect
to different values of smoothing parameter $\epsilon$ (blue dots) are shown in Figure~\ref{fig:bc_smooth_opt}(a). Dashed line
represents the result of optimization without smoothing, i.e.~when $\epsilon=0$. First, we conclude that the positive effect of
smoothing mixed boundary conditions is seen for $10^{-4} < \epsilon < 10^1$. In fact, reduction of $\mJ$ values does not allow to
conclude on improvement made for both controls $\sigma$ and $U$ individually. In order to do this and to identify optimal value
for $\epsilon$ parameter, we examine additionally $\sigma$ and $U$ solution norms
$N_{\sigma} = \frac{\| \sigma - \sigma_{true}\|_{L_2}}{\| \sigma_{true}\|_{L_2}}$ and
$N_U = \frac{\| U - U_{true}\|_{L_2}}{\| U_{true}\|_{L_2}}$ presented in Figure~\ref{fig:bc_smooth_opt}(b). We pick values
(shown by hexagons) for the best results obtained at $\epsilon^* = 0.3162$ with the maximum of the performance in terms of
improving solutions for both controls $\sigma$ and $U$ evaluated respectively as $1.82\%$ and $1.0\%$.
\begin{figure}[!htb]
  \begin{center}
  \mbox{
  \subfigure[]{\includegraphics[width=0.50\textwidth]{Figs/bc_smooth_obj}}
  \subfigure[]{\includegraphics[width=0.50\textwidth]{Figs/bc_smooth_sol_norm}}}
  \caption{(a) Cost functional $\mJ$ values and (b) solution norms
    $N_{\sigma} = \frac{\| \sigma - \sigma_{true}\|_{L_2}}{\| \sigma_{true}\|_{L_2}}$ and
    $N_U = \frac{\| U - U_{true}\|_{L_2}}{\| U_{true}\|_{L_2}}$ evaluated at termination (dots) for different
    values of smoothing parameter $\epsilon$ and (dashed lines) without smoothing ($\epsilon=0$).
    The best results obtained at $\epsilon^* = 0.3162$ are shown by hexagons.}
  \label{fig:bc_smooth_opt}
  \end{center}
\end{figure}

The improved regularity of the discretized gradients $\nabla_U \mJ$, and thus their overall quality, could be also confirmed
by re-running the validation tests described in Section~\ref{sec:kappa_test} using optimal value $\epsilon^* = 0.3162$.
The new results are presented in Figure~\ref{fig:kappa_test_U} in red color. As seen in Figure~\ref{fig:kappa_test_U}(a),
new gradients $\nabla_U \mJ(\sigma,U)$ computed with smoothed boundary conditions show significantly lesser error
demonstrated by the plateau formed by $\kappa$-values which is now moved much closer to the unity. This is also supported
by the diagnostic test applied individually to every component $U_l$. As clearly observed in Figure~\ref{fig:kappa_test_U}(b),
the new result (red dots) shows increased sensitivity of cost functional $\mJ (\sigma,U)$ to changes in boundary potentials
$U_l$ at individual electrodes $E_l$ in the majority of 16 cases.
